# Supplementary material for: Electronic structure and magnetic properties of Gd-doped and Eu-rich EuO
Source: arXiv:1308.1223 source file (2013-08-06)
Supplement: Supplementary file 1 [file Supplementary.pdf]

# Supplemental material: Effect of Gd doping and O vacancies on the Curie temperature of EuO: A magnetostructural cluster expansion approach

J. M. An and K. D. Belashchenko
*Department of Physics and Astronomy and Nebraska Center for Materials and Nanoscience, University of Nebraska–Lincoln, Lincoln, Nebraska 68588, USA*
(Dated: December 11, 2012)

## I. INPUT CONFIGURATIONS FOR GD-DOPED EUO

86 single-site spin-flip configurations close to the ground state FM configuration were used to fit the parameters in the magnetostructural cluster expansion, let alone 8 random spin configurations to assess non-Heisenberg contributions. A total of 42 supercell structures were constructed over the Gd composition range $x$=0−0.25 of $Gd_xEu_{1-x}O$, and the explicit compositions are $x$= 1/32, 2/32, 3/32, 2/16, 1/8, 3/16, 2/8, 1/4, where the numerator is the number of Gd atoms and the denomenator the total number of cations in supercells. In each of the structures, we considered symmetrically nonequivalent Gd or Eu sites, and Eu sites at varying distances from impurity Gd sites for the spin-flip energy calculations. All single-site spin-flip energies are denoted by $E_{spin}$ in units of meV/spin, and the total number of *first (second) nearest Gd neigbors* of the spin-flipped site is specified by $N_1$ ($N_2$). $T_i$ for $i = 1, 2, 3$ are supercell lattice vectors and are specified, together with atomic positions R, in units of fcc conventional unit-cell lattice constant 'a'. A 2×2×2 cubic supercell of stoichiometric EuO containing 32 Eu cations is shown in Structure 1 at x=0/32 below.

### A. x=0/32

Structure 1 :
$T_1$=(2,0,0), $T_2$=(0,2,0), $T_3$=(0,0,2)

| Species | R | $N_1$ | $N_2$ | $E_{spin}$ |
|---|---|---|---|---|
| Eu | (0,0,0) | 0 | 0 | 46.7 |

### B. x=1/32

Structure 2 :
$T_1$=(2,0,0), $T_2$=(0,2,0), $T_3$=(0,0,2)

| Species | R | $N_1$ | $N_2$ | $E_{spin}$ |
|---|---|---|---|---|
| Gd | (1,1,1) | 0 | 0 | 36.5 |
| Eu | (1/2,1/2,1) | 1 | 0 | 66.3 |
| Eu | (0,1,1) | 0 | 2 | 71.8 |
| Eu | (0,0,0) | 0 | 0 | 67.1 |

### C. x=2/32

Structure 3 :
$T_1$=(2,0,0), $T_2$=(0,2,0), $T_3$=(0,0,2)
Gd: (1,1,1), (1/2,1/2,1)

| Species | R | $N_1$ | $N_2$ | $E_{spin}$ |
|---|---|---|---|---|
| Gd | (1,1,1) | 1 | 0 | 49.7 |
| Eu | (0,0,1) | 1 | 0 | 85.4 |
| Eu | (1,0,1) | 1 | 2 | 91.2 |
| Eu | (3/2,3/2,0) | 0 | 0 | 81.1 |

Structure 4 :
$T_1$=(2,0,0), $T_2$=(0,2,0), $T_3$=(0,0,2)
Gd: (1,1,1), (0,1,1)

| Species | R | $N_1$ | $N_2$ | $E_{spin}$ |
|---|---|---|---|---|
| Gd | (1,1,1) | 0 | 2 | 65.6 |
| Eu | (1/2,1/2,1) | 2 | 0 | 81.7 |
| Eu | (1,0,1) | 0 | 2 | 94.2 |
| Eu | (3/2,1/2,0) | 0 | 0 | 80.9 |
| Eu | (1,0,0) | 0 | 0 | 82.8 |

Structure 5 :
$T_1$=(2,0,0), $T_2$=(0,2,0), $T_3$=(0,0,2)
Gd: (1,1,1), (0,0,0)

| Species | R | $N_1$ | $N_2$ | $E_{spin}$ |
|---|---|---|---|---|
| Gd | (1,1,1) | 0 | 0 | 49.1 |
| Eu | (1/2,1/2,1) | 1 | 0 | 81.7 |
| Eu | (0,1,1) | 0 | 2 | 94.0 |

Structure 6 :
$T_1$=(2,0,0), $T_2$=(0,2,0), $T_3$=(0,0,2)
Gd: (1,0,1), (0,1,1)

| Species | R | $N_1$ | $N_2$ | $E_{spin}$ |
|---|---|---|---|---|
| Eu | (1/2,3/2,1) | 2 | 0 | 84.2 |
| Eu | (1,1,1) | 0 | 4 | 105.8 |
| Eu | (3/2,0,1/2) | 1 | 0 | 80.8 |

### D. x=3/32

Structure 7 :
$T_1$=(2,0,0), $T_2$=(0,2,0), $T_3$=(0,0,2)
Gd: (1,1,1), (0,1,1), (0,0,0)

| Species | R | $N_1$ | $N_2$ | $E_{spin}$ |
|---|---|---|---|---|
| Gd | (1,1,1) | 0 | 2 | 78.9 |
| Eu | (0,0,1) | 0 | 4 | 122.6 |
| Eu | (1,0,0) | 0 | 2 | 102.2 |

### E. x=2/16

Structure 8 :
$T_1$=($\sqrt{2}$,0,0), $T_2$=(0,$\sqrt{2}$,0), $T_3$=(0,0,2)
Gd: (0,0,0), (1/$\sqrt{2}$,1/$\sqrt{2}$,1)

| Species | R | $N_1$ | $N_2$ | $E_{spin}$ |
|---|---|---|---|---|
| Gd | (0,0,0) | 0 | 0 | 78.8 |
| Eu | (1/2$\sqrt{2}$,1/2$\sqrt{2}$,1/2) | 2 | 0 | 91.6 |
| Eu | (1/$\sqrt{2}$,1/$\sqrt{2}$,0) | 0 | 6 | 140.4 |

Structure 9 :
$T_1$=(2,0,0), $T_2$=(0,2,0), $T_3$=(0,0,1)
Gd: (0,1,0), (1,0,0)

| Species | R | $N_1$ | $N_2$ | $E_{spin}$ |
|---|---|---|---|---|
| Gd | (0,1,0) | 0 | 2 | 74.8 |
| Eu | (1/2,1/2,0) | 2 | 0 | 86.9 |
| Eu | (0,0,0) | 0 | 4 | 124.1 |

Structure 10 :
$T_1$=(2,0,0), $T_2$=(0,2,0), $T_3$=(0,0,1)
Gd: (1,1,0), (3/2,3/2,0)

| Species | R | $N_1$ | $N_2$ | $E_{spin}$ |
|---|---|---|---|---|
| Gd | (1,1,0) | 1 | 2 | 73.9 |
| Eu | (1/2,1/2,0) | 1 | 0 | 95.4 |
| Eu | (3/2,1/2,0) | 1 | 2 | 104.1 |
| Eu | (3/2,1,1/2) | 4 | 0 | 82.6 |

Structure 11 :
$T_1$=(2,0,0), $T_2$=(0,2,0), $T_3$=(0,0,1)
Gd: (1,1,0), (1,0,0)

| Species | R | $N_1$ | $N_2$ | $E_{spin}$ |
|---|---|---|---|---|
| Gd | (1,1,0) | 0 | 4 | 90.8 |
| Eu | (3/2,1,1/2) | 2 | 0 | 80.6 |
| Eu | (0,0,0) | 0 | 2 | 105.8 |

Structure 12 :
$T_1$=($\sqrt{2}$,0,0), $T_2$=(0,$\sqrt{2}$,0), $T_3$=(0,0,2)
Gd: (0,0,0), (0,1/$\sqrt{2}$,0)

| Species | R | $N_1$ | $N_2$ | $E_{spin}$ |
|---|---|---|---|---|
| Gd | (0,0,0) | 2 | 0 | 63.8 |
| Eu | (1/$\sqrt{2}$,0,0) | 2 | 4 | 109.3 |

Structure 13 :
$T_1$=($\sqrt{2}$,0,0), $T_2$=(0,$\sqrt{2}$,0), $T_3$=(0,0,2)
Gd: (0,0,0), (1/$\sqrt{2}$,1/$\sqrt{2}$,0)

| Species | R | $N_1$ | $N_2$ | $E_{spin}$ |
|---|---|---|---|---|
| Gd | (0,0,0) | 0 | 4 | 93.3 |
| Eu | (3/2$\sqrt{2}$,1/2$\sqrt{2}$,1/2) | 2 | 0 | 85.4 |
| Eu | (0,1/$\sqrt{2}$,1) | 0 | 0 | 87.7 |
| Eu | (1/$\sqrt{2}$,1/$\sqrt{2}$,1) | 0 | 2 | 109.6 |

### F. x=1/8

Structure 14 :
$T_1$=(1,1,1), $T_2$=(-1,1,-1), $T_3$=(-1/2,0,1/2)

| Species | R | $N_1$ | $N_2$ | $E_{spin}$ |
|---|---|---|---|---|
| Gd | (0,0,0) | 2 | 0 | 67.4 |

Structure 15 :
$T_1$=(1/2,-1,-1/2), $T_2$=(1/2,-1,1/2), $T_3$=(-2,0,0)

| Species | R | $N_1$ | $N_2$ | $E_{spin}$ |
|---|---|---|---|---|
| Gd | (0,0,0) | 0 | 2 | 79.8 |

Structure 16 :
$T_1$=(-1/2,1/2,1), $T_2$=(1/2,1,-1/2), $T_3$=(-1,0,-1)

| Species | R | $N_1$ | $N_2$ | $E_{spin}$ |
|---|---|---|---|---|
| Gd | (0,0,0) | 0 | 0 | 64.2 |

Structure 17 :
$T_1$=(1/2,1,-1/2), $T_2$=(1/2,-1,-1/2), $T_3$=(-1,0,-1)

| Species | R | $N_1$ | $N_2$ | $E_{spin}$ |
|---|---|---|---|---|
| Gd | (0,0,0) | 0 | 0 | 67.1 |

Structure 18 :
$T_1$=(1,-1,0), $T_2$=(0,-1,-1), $T_3$=(1/2,1,-1/2)

| Species | R | $N_1$ | $N_2$ | $E_{spin}$ |
|---|---|---|---|---|
| Gd | (0,0,0) | 0 | 0 | 73.4 |

Structure 19 :
$T_1$=(1/2,1,-1/2), $T_2$=(-1/2,0,-1/2), $T_3$=(-3/2,1,3/2)

| Species | R | $N_1$ | $N_2$ | $E_{spin}$ |
|---|---|---|---|---|
| Gd | (0,0,0) | 2 | 0 | 64.3 |

Structure 20 :

$T_1$=(1/2,0,3/2), $T_2$=(3/2,0,-1/2), $T_3$=(0,1,0)

| Species | R | $N_1$ | $N_2$ | $E_{spin}$ |
|---|---|---|---|---|
| Gd | (0,0,0) | 0 | 2 | 80.0 |

Structure 21 :
$T_1$=(-1/2,-1/2,-2), $T_2$=(1/2,1/2,-2), $T_3$=(1/2,-1/2,2)

| Species | R | $N_1$ | $N_2$ | $E_{spin}$ |
|---|---|---|---|---|
| Gd | (0,0,0) | 0 | 4 | 85.2 |

Structure 22 :
$T_1$=(0,-1,0), $T_2$=(-1,0,0), $T_3$=(0,0,-2)

| Species | R | $N_1$ | $N_2$ | $E_{spin}$ |
|---|---|---|---|---|
| Gd | (0,0,0) | 0 | 4 | 99.8 |

Structure 23 :
$T_1$=(-1,-1,0), $T_2$=(-1,1,0), $T_3$=(0,0,-1)

| Species | R | $N_1$ | $N_2$ | $E_{spin}$ |
|---|---|---|---|---|
| Gd | (0,0,0) | 0 | 2 | 84.9 |

Structure 24 :
$T_1$=(-1,0,-1), $T_2$=(0,-1,-1), $T_3$=(-1,-1,0)

| Species | R | $N_1$ | $N_2$ | $E_{spin}$ |
|---|---|---|---|---|
| Gd | (0,0,0) | 0 | 0 | 79.0 |

Structure 25 :
$T_1$=(-1/2,-1/2,2), $T_2$=(-1/2,-1/2,-2), $T_3$=(1/2,-1/2,0)

| Species | R | $N_1$ | $N_2$ | $E_{spin}$ |
|---|---|---|---|---|
| Gd | (0,0,0) | 2 | 0 | 63.0 |

Structure 26 :
$T_1$=(1/2,-1/2,0), $T_2$=(-1,-1,0), $T_3$=(0,0,-2)

| Species | R | $N_1$ | $N_2$ | $E_{spin}$ |
|---|---|---|---|---|
| Gd | (0,0,0) | 2 | 0 | 68.8 |

Structure 27 :
$T_1$=(-1,1,1), $T_2$=(-3/2,1/2,0), $T_3$=(-1/2,-1/2,1)

| Species | R | $N_1$ | $N_2$ | $E_{spin}$ |
|---|---|---|---|---|
| Gd | (0,0,0) | 0 | 0 | 66.4 |

Structure 28 :
$T_1$=(0,-1/2,1/2), $T_2$=(1,0,0), $T_3$=(0,2,2)

| Species | R | $N_1$ | $N_2$ | $E_{spin}$ |
|---|---|---|---|---|
| Gd | (0,0,0) | 2 | 2 | 74.7 |

### G. x=2/12

Structure 29 :
$T_1$=(-1/2,0,1/2), $T_2$=(1,1,1), $T_3$=(-1,2,-1)
Gd: (0,0,0), (-1/2,1/2,0)

| Species | R | $N_1$ | $N_2$ | $E_{spin}$ |
|---|---|---|---|---|
| Eu | (1/12,1/3,7/12) | 3 | 2 | 96.4 |

Structure 30 :
$T_1$=(-1/2,0,1/2), $T_2$=(1,1,1), $T_3$=(-1,2,-1)
Gd: (1/3,1/3,1/3), (-1/2,1/2,0)

| Species | R | $N_1$ | $N_2$ | $E_{spin}$ |
|---|---|---|---|---|
| Eu | (0,0,0) | 4 | 0 | 73.0 |
| Gd | (1/3,1/3,1/3) | 3 | 2 | 63.8 |

Structure 31 :
$T_1$=(-1/2,0,1/2),$T_2$=(1,1,1),$T_3$=(-1,2,-1)
Gd: (-1,3/2,-1/2), (1/12,1/3,7/12)

| Species | R | $N_1$ | $N_2$ | $E_{spin}$ |
|---|---|---|---|---|
| Gd | (-1,3/2,-1/2) | 2 | 1 | 79.7 |

Structure 32 :
$T_1$=(-1/2,0,1/2),$T_2$=(1,1,1),$T_3$=(-1,2,-1)
Gd: (-1/2,1,-1/2), (1/12,1/3,7/12)

| Species | R | $N_1$ | $N_2$ | $E_{spin}$ |
|---|---|---|---|---|
| Gd | (-1/2,1,-1/2) | 2 | 0 | 72.3 |

Structure 33 :
$T_1$=(-1/2,1/2,1),$T_2$=(0,1,-1),$T_3$=(-3/2,-1,-1/2)
Gd: (-3/2,-1/2,0), (0,1/2,-1/2)

| Species | R | $N_1$ | $N_2$ | $E_{spin}$ |
|---|---|---|---|---|
| Gd | (-3/2,-1/2,0) | 1 | 2 | 82.6 |

Structure 34 :
$T_1$=(-1/2,1/2,1),$T_2$=(0,1,-1),$T_3$=(-3/2,-1,-1/2)
Gd: (-1,-1/2,-1/2), (0,0,0)

| Species | R | $N_1$ | $N_2$ | $E_{spin}$ |
|---|---|---|---|---|
| Gd | (-1,-1/2,-1/2) | 1 | 0 | 68.5 |

Structure 35 :
$T_1$=(-1/2,1/2,1),$T_2$=(0,1,-1),$T_3$=(-3/2,-1,-1/2)
Gd: (-1,-7/12,-3/4), (0,1/2,-1/2)

| Species | R | $N_1$ | $N_2$ | $E_{spin}$ |
|---|---|---|---|---|
| Gd | (-1,-7/12,-3/4) | 1 | 0 | 67.6 |

Structure 36 :
$T_1$=(-1/2,1/2,1),$T_2$=(0,1,-1),$T_3$=(-3/2,-1,-1/2)
Gd: (-1,0,0), (0,0,0)

| Species | R | $N_1$ | $N_2$ | $E_{spin}$ |
|---|---|---|---|---|
| Gd | (-1,0,0) | 0 | 1 | 70.7 |

### H. x=3/16

Structure 37 :
$T_1$=($\sqrt{2}$,0,0),$T_2$=(0,$\sqrt{2}$,0),$T_3$=(0,0,2)
Gd: (0,0,0), (0,1/$\sqrt{2}$,1), (0,0,1)

| Species | R | $N_1$ | $N_2$ | $E_{spin}$ |
|---|---|---|---|---|
| Eu | (1/$\sqrt{2}$,1/$\sqrt{2}$,0) | 0 | 6 | 134.7 |
| Gd | (0,0,0) | 0 | 2 | 99.8 |
| Gd | (0,1/$\sqrt{2}$,1) | 0 | 4 | 107.3 |
| Gd | (0,0,1) | 0 | 6 | 154.4 |

Structure 38 :
$T_1$=($\sqrt{2}$,0,0),$T_2$=(0,$\sqrt{2}$,0),$T_3$=(0,0,2)
Gd: (0,0,0), (1/$\sqrt{2}$,1/$\sqrt{2}$,1), (0,1/$\sqrt{2}$,1)

| Species | R | $N_1$ | $N_2$ | $E_{spin}$ |
|---|---|---|---|---|
| Eu | (1/$\sqrt{2}$,0,0) | 2 | 0 | 100.7 |
| Eu | (0,1/$\sqrt{2}$,0) | 2 | 2 | 102.6 |
| Eu | (0,0,1) | 0 | 6 | 128.6 |
| Gd | (0,0,0) | 0 | 0 | 80.8 |
| Gd | (1/$\sqrt{2}$,1/$\sqrt{2}$,1) | 2 | 0 | 78.8 |
| Gd | (0,1/$\sqrt{2}$,1) | 2 | 0 | 62.0 |

Structure 39 :
$T_1$=($\sqrt{2}$,0,0),$T_2$=(0,$\sqrt{2}$,0),$T_3$=(0,0,2),
Gd: (0,0,0), (1/$\sqrt{2}$,1/$\sqrt{2}$,1), (1/2$\sqrt{2}$,1/2$\sqrt{2}$,1/2)

| Species | R | $N_1$ | $N_2$ | $E_{spin}$ |
|---|---|---|---|---|
| Gd | (0,0,0) | 1 | 0 | 79.5 |
| Gd | (1/2$\sqrt{2}$,1/2$\sqrt{2}$,1/2) | 2 | 0 | 66.4 |
| Eu | (0,0,1) | 1 | 6 | 136.5 |

Structure 40 :
$T_1$=(2,0,0), $T_2$=(0,2,0), $T_3$=(0,0,1)
Gd: (0,1,0), (1,0,0), (1,1,0)

| Species | R | $N_1$ | $N_2$ | $E_{spin}$ |
|---|---|---|---|---|
| Gd | (0,1,0) | 0 | 4 | 102.1 |
| Gd | (1,1,0) | 0 | 6 | 138.2 |

### I. x=2/8

Structure 41 :
$T_1$=(1,0,0), $T_2$=(0,1,0), $T_3$=(0,0,2)
Gd: (0,0,0), (1/2,1/2,1)

| Species | R | $N_1$ | $N_2$ | $E_{spin}$ |
|---|---|---|---|---|
| Eu | (0,1/2,1/2) | 4 | 0 | 72.2 |
| Eu | (1/2,1/2,0) | 4 | 2 | 91.2 |
| Gd | (1/2,1/2,1) | 0 | 4 | 78.2 |

### J. x=1/4

Structure 42 :
$T_1$=(0,0,1), $T_2$=(0,1,0), $T_3$=(-1,0,0)

| Species | R | $N_1$ | $N_2$ | $E_{spin}$ |
|---|---|---|---|---|
| Eu | (0,0,0) | 4 | 0 | 72.2 |
| Gd | (-1/2,0,1/2) | 0 | 6 | 96.2 |
